# Supplementary material for: Time-Optimal Online Replanning for Agile Quadrotor Flight
Source: arXiv:2203.09839 source file (2022-07-21)
Supplement: Supplementary file 1 [file appendix.tex]

\subsection*{Supplementary Materials}
